# Supplementary material for: Partitioned Variational Inference: A Framework for Probabilistic Federated Learning
Source: arXiv:2202.12275 source file (2022-04-28)
Supplement: Supplementary file 1 [file appendix_optim.tex]

\section{Stochastic Approximations of Fixed-Point / Natural Gradient Updates}

\subsection{Stochastic mini-batch approximation}
\label{section:optim:mini-batch}

There are two distinct ways to apply stochastic approximations within the PVI scheme. 

\subsubsection{Stochastic Approximation within the Local Free-Energy}
\label{sec:optim:stoc_approx_1}

The first form of stochastic approximation leverages the fact that each local free-energy decomposes into a sum over data points and can, therefore, be approximated by sampling mini-batches within each data partition $\bfy_m$. In the case where each partition includes a large number of data points, this leads to algorithms that converge more quickly than the batch variants---since a reasonable update for the approximate posterior can often be determined from just a few data points---and this faster convergence opens the door to processing larger data sets.

Mini-batch approximation can be employed in the general PVI case, but for simplicity we consider the global VI case here $M=1$. If simplified fixed point updates are used for optimization, then sampling $L$ mini-batches of data from the data distribution $\mathbf{y}_l \stackrel{\text{iid}}{\sim} p_{\text{data}}(y)$ yields the following stochastic approximation to the damped updates,\footnote{We have used a distinct notation for a mini-batch ($\bfy_l$) and a data group ($\bfy_m$) since the former will be selected iid from the data set and will vary at each epoch, whilst the latter need not be determined in this way and is fixed across epochs.}
\begin{align}
\*\eta^{(i)}_{q}  &
= (1-\rho)\*\eta^{(i-1)}_{q} + \rho \left ( \*\eta_0 + L \frac{\mathrm{d}}{\mathrm{d}\*\mu_q} \mathbb{E}_q \left[\log p(\bfy_l|\*\theta)\right] \right),\\
& = \*\eta^{(i-1)}_{q} + \rho' \left (   \frac{\mathrm{d}}{\mathrm{d}\*\mu_q} \mathbb{E}_q \left[\log p(\bfy_l|\*\theta)\right] - \*\eta^{(i-1)}_{\text{like}}/L \right).
\label{eq:stoch-global-main}
\end{align}
Here the first form of the update is stochastic natural gradient ascent and the second form reveals the implied deletion step where $\*\eta^{(i-1)}_{\text{like}}/L = (\*\eta^{(i-1)}_{q} - \*\eta^{(i-1)}_{0})/L$ is the contribution a mini-batch likelihood makes to the posterior natural parameters on average. The rescaled learning rate is $\rho' = L \rho$. These two forms reveals that the mini-batch stochastic natural gradient update resembles an EP update step. See appendix \ref{sec:stochastic-approx} for full details.

\subsubsection{Stochastic Scheduling of Updates Between Local Free-Energies} 
\label{sec:optim:stoc_approx_2}

The second form of stochastic approximation is to randomize the update schedule. For example, using $M=N$ and randomly selecting subsets of data to update in parallel. This can be memory intensive, requiring $N$ local natural parameters to be stored. A more memory efficient approach is to fix the mini-batches across epochs and to visit the data groups $\bfy_m$ in a random order \citep{khan+li:2018}. For the simplified fixed point updates, this yields  
\begin{align}
\*\eta^{(i)}_{m}  & = (1-\rho) \*\eta^{(i-1)}_{m} + \rho \frac{\mathrm{d}}{\mathrm{d}\*\mu_{q^{(i-1)}}} \Exp{q^{(i-1)}}{\log p(\bfy_{m}|\*\theta)}. \label{eq:stoch-local-main}
\end{align}
This approach results in a subtly different update to $q$ that retains a specific approximation to the likelihood of each data partition, rather than a single global approximation
\begin{align}
\*\eta^{(i)}_{q}  &
= \*\eta^{(i-1)}_{q} - \rho \left ( \frac{\mathrm{d}}{\mathrm{d}\*\mu_q} \Exp{q}{\log p(\bfy_m|\*\theta)} - \*\eta^{(i-1)}_{q} \right).\label{eq:stoch-local-EP-main}
\end{align}
If the first approach in \eqref{eq:stoch-local-main} employs learning rates that obey the Robins Munro conditions, the fixed points will be identical to the second approach in \eqref{eq:stoch-local-EP-main} and they will correspond to optima of the global free-energy.

\subsubsection{Comparing and Contrasting Stochastic Approaches} 
\label{sec:optim:comparing_stoc}

There are pros and cons to both approaches. The first approach in \Cref{sec:optim:stoc_approx_1} has a memory footprint $L$ times smaller than the second approach in \Cref{sec:optim:stoc_approx_2} and can converge more quickly. For example, on the first pass through the data, it effectively allows approximate likelihoods for as of yet unseen data to be updated based on those for the data seen so far, which means that larger learning rates can be used $\rho' > \rho$. The second approach is required for continual learning, asynchronous updates, and client-side processing where the assumption that each mini-batch is iid (and a single gradient step is performed on each) is typically incorrect. The second approach also tends to produce less noisy learning curves, with stochasticity only entering via the schedule and not as an approximation to the local free-energy and the gradients thereof. 

These approaches could also be combined, with stochastic scheduling selecting the local free-energy to update next and mini-batch updates employed for each local free-energy optimization. See appendix \ref{sec:stochastic-approx} for a full discussion.
